# Supplementary material for: From Prompts to Pavement: LMMs-based Agentic Behavior-Tree Generation Framework for Autonomous Vehicles
Source: arXiv:2601.12358 source file (2026-01-18)
Supplement: Supplementary file 1 [file Appendix.tex]

\appendices
\section{Proof of the First Zonklar Equation}
Appendix one text goes here.

% you can choose not to have a title for an appendix
% if you want by leaving the argument blank
\section{}
Appendix two text goes here.
